# Supplementary material for: Impact of Nitrogen and Oxygen Interstitials on Niobium SRF Cavity Performance
Source: arXiv:2509.18564 source file (2026-01-21)
Supplement: Supplementary file 1 [file Supplementary_Material.pdf]

# SUPPLEMENTARY MATERIALS

## Impact of Nitrogen and Oxygen Interstitials on Niobium SRF Cavity Performance

H. Hu<sup>\*1,2</sup>, Y.-K. Kim<sup>1,2</sup>, J. Lee<sup>2</sup>, and D. Bafia<sup>†2</sup>

<sup>1</sup>Physics Department, The University of Chicago, Chicago, Illinois, 60637, USA

<sup>2</sup>Fermi National Accelerator Laboratory, Batavia, Illinois 60510, USA

September 19, 2025

### 1 Time-of-Flight Secondary Ion Mass Spectroscopy (ToF-SIMS)

Each reported impurity depth profile represents the average of three  $200\text{ }\mu\text{m} \times 200\text{ }\mu\text{m}$  regions per sample. To minimize edge effects, the sputter crater for each spot is  $600\text{ }\mu\text{m} \times 600\text{ }\mu\text{m}$ . A  $2\text{ keV CS}^+$  ion beam was used for sputtering. The analysis chamber pressure was maintained below  $4 \times 10^{-10}$  mbar and the heating chamber pressure below  $1 \times 10^{-7}$  mbar. Implanted N and O standards were measured in parallel to calibrate the relative ToF-SIMS intensity to absolute concentration[1].  $\text{O}^-$  and  $\text{NbN}^-$  signals were used to quantify the relative sensitivity factors (RSFs) for O and N, respectively. The average RSF values with respect to Nb were  $1.25 \pm 0.43 \times 10^{21}$  ions/ $\text{cm}^3$  for N and  $2.07 \pm 0.55 \times 10^{20}$  ions/ $\text{cm}^3$  for O. Reported uncertainties account for variations in chamber pressure, emission current, sputtering rate across all measurement sessions. Sputtering depth was calibrated relative to the 5 nm Nb pentoxide layer, determined by the point at which  $\text{Nb}_2\text{O}_5$  counts drop below 10 counts[2]. For *in-situ* baked samples, the pentoxide layer may be partially dissolved; in such cases, a reference sample with a fully intact oxide was used for depth calibration. The ToF-SIMS system exhibited background levels of  $60 \pm 8$  atomic ppm (ppma) for N and  $270 \pm 40$  ppma for O, which represent the effective detection limits of the measurements.

---

<sup>\*</sup>hannahhu@uchicago.edu

<sup>†</sup>dbafia@fnal.gov

## 2 Atom Probe Tomography (APT)

APT measurements were carried out on a CAMECA LEAP5000XS at 40 K in UHV ( $1 \times 10^{-11}$  Torr). A 355 nm ultraviolet laser was used for field evaporation, operated from 30 pJ to 45 pJ with a repetition rate of 500 kHz. The detection rate was maintained between 0.3–0.5%, with an overall atomic detection efficiency of 80%. With sub-nm spatial resolution, APT revealed a nitrogen-rich band on one side of the sample, where the local concentration is about five times higher than the surrounding regions. This feature is likely associated with a grain boundary; given that the grain size in this sample exceeds 50  $\mu\text{m}$ , a boundary effect is unlikely to strongly influence the average concentration across the entire cavity surface [3]. Elevated oxygen counts were also observed on the left side of the sample, coinciding with an enhanced hydrogen signal in the same region. This can be attributed the relatively high laser pulse energy of 45 pJ causing redistribution effects of H and O from water vapor within the system [4]. To minimize such artifacts, analysis was restricted to a region of interest outside both the N-enriched band and the laser-affected zone. Within this region, the average N concentration was  $870 \pm 150$  ppma. The same sample later measured with ToF-SIMS yielded average N concentration of  $730 \pm 290$  ppma, corresponding to a Z-score of 0.43. O quantification is more challenging since signal from interstitial O is convoluted with suboxide contributions dominating the near-surface signal. Deeper in the bulk, once the suboxide effects disappear, a direct comparison of the average concentration from a depth of 220 nm to 240 nm gives  $200 \pm 30$  ppma for APT and  $180 \pm 60$  ppma for ToF-SIMS, corresponding to a Z-score of 0.30.

## References

- [1] A. Budrevich and J. Hunter, AIP Conference Proceedings **449**, 169 (1998).
- [2] D. Bafia, Exploring and Understanding the Limitations of Niobium SRF Cavity Performance, Ph.D. thesis, Illinois Institute of Technology (2020).
- [3] E. M. Lechner, J. W. Angle, C. Baxley, M. J. Kelley, and C. E. Reece, Phys. Rev. Accel. Beams **26**, 103101 (2023)
- [4] Y.-J. Kim and D. N. Seidman, Microscopy and Microanalysis **21**, 535 (2015).
